# Supplementary material for: Stochastic and Deterministic Vector Chromatography of Suspended Particles in 1D-Periodic Potentials
Source: arXiv:1110.2670 ancillary file (2011-10-12)
Supplement: Supplementary file 1 [file supp_info.pdf]

# Supplementary information

October 12, 2011

### Experimental system and methods

All the data presented in the manuscript, and summarized in Table **??** below, was obtained using the same patterned substrate: a microscope glass slide with an array of grooves 65 nm deep obtained by wet etching under sonication in a 1:200 solution of Hydrofloric (HF) acid (50 % v/v) in water. A positive photoresist (*Shipley* S1813) was used as a mask for the HF etching.

The experiments were performed using a casing that could be disassembled to facilitate the cleaning and reuse of the same substrate. The patterned substrate is closed with a PDMS cover containing fluidic channels that are 500 $\mu$m tall. The patterned glass substrate and the PDMS cover are then sandwiched between two plexiglass plates that are fastened with screws to apply pressure and seal the device.

The device is first primed with a 0.1 mM KOH solution and mounted on an upright microscope with transmitted illumination. A sparse stream of settled particles is then flow focused in the middle of the 5 mm wide channel towards the pattern of grooves. The grooves are fabricated at an angle of 45° with respect to the direction of the flow. After the first particles in the focused stream reach the grooves, all inlet and outlet ports of the device are closed and the microscope is then tilted to the desired angle to allow gravity to drive the particles.

Silica particles with nominal diameters of 2.14 and 4.32 $\mu$m and polystyrene particles with a nominal diameter of 4.31 $\mu$m (Bangs Laboratories, Inc.) were used as received. All particles have a specified coefficient of variation between 10–15 %. Suspensions were prepared diluting the particles with a 0.1 mM KOH solution.

Only one kind of particle was used in each experiment to facilitate the analysis. The field of view captured both an unmodified region of the glass surface, as well as a region with grooves, with horizontal spans for a typical experiment of 250 $\mu$m and 600 $\mu$m, respectively. The particles were tracked using *PolyParticleTracker* [**?**] and the forcing and trajectory angles were obtained by fitting a straight line to the trajectory of each particle. Only particles with trajectories with a horizontal displacement longer than half of the horizontal span of the patterned region where considered for the measurement of the trajectory angle. The resulting mean and standard deviation are reported in Table **??**. The value of the standard deviation reported for the deflection angle correspond to the

Table 1: Experimental data

| | $\theta_t$ | | $\theta_F$ | | | $\Delta\theta = \theta_t - \theta_F$ | | |
|---|---|---|---|---|---|---|---|---|
| | mean | std | mean | std | $N$ | mean | std | $N$ |
| Silica 4.32 $\mu$m | 0.8 | 0.1 | 46 | 6 | 75 | 31 | 23 | 183 |
| | 1.3 | 0.2 | 48 | 6 | 91 | 25 | 20 | 239 |
| | 2.7 | 0.3 | 46 | 3 | 23 | 9 | 7 | 28 |
| | 3.6 | 0.4 | 46 | 3 | 29 | 6 | 12 | 43 |
| | 4.0 | 0.1 | 48 | 3 | 125 | 5 | 7 | 339 |
| | 4.16 | 0.08 | 44 | 3 | 19 | 2 | 9 | 25 |
| | 4.4 | 0.4 | 47 | 3 | 45 | 2 | 6 | 52 |
| Silica 2.14 $\mu$m | 1.0 | 0.4 | 39 | 13 | 18 | 2 | 30 | 28 |
| | 2.6 | 0.4 | 44 | 8 | 135 | 3 | 17 | 177 |
| | 6.3 | 0.3 | 50 | 7 | 38 | -1 | 14 | 100 |
| Polystyrene 4.31 $\mu$m | 0.7 | 0.3 | 41 | 15 | 69 | 5 | 27 | 105 |
| | 1.9 | 0.5 | 46 | 16 | 19 | 4 | 32 | 48 |
| | 5.6 | 0.3 | 43 | 7 | 57 | -1 | 14 | 95 |
| | 6.5 | 0.4 | 43 | 8 | 38 | -1 | 16 | 65 |

sum of standard deviations of the forcing and the trajectory angles.

### Order of magnitude estimate of the width of the transition region

The data for the deflection angle of the 4.31 $\mu$m silica particles was fitted to the analytical result obtained for the *dichotomous potential with linear transitions* (LTD potential) using the width of the transition region as a fitting parameter. The fitting was done using a Levenberg-Marquardt algorithm. For comparison, we estimate the order of magnitude of the width of the transition region using the concept of a *zone of influence* [**?**] for a particle of radius $a$ suspended at its equilibrium separation from the wall, $h_e$, and in the vicinity of a step of height $\Delta\mathcal{H}$. In the calculation, a particle at its equilibrium separation from the wall is located at a distance $D$ from the sharp step, such that a shell of thickness $h_e + \kappa^{-1}$, where $\kappa^{-1}$ is the Debye length, touches the corner of the step. The distance $D$ corresponds to half of the width of the transition region $\delta_{zoi} = 2\sqrt{2(a + h_e)(\Delta\mathcal{H} + \kappa^{-1})}$. To calculate $h_e$, the form and parameters of the electrostatic and Van der Waals interaction potentials were taken from the literature. In the notation of reference [**?**], the Stern potentials for the glass substrate and the silica particles were taken to be $\psi_s = \psi_p = -60$ mV, and the Van der Waals prefactor $A$ and exponent $p$ were taken to be 2 nm and 2, respectively. The diameter of the particles was taken to be their nominal value of 4.32 $\mu$m and the density was 1.96 g/mL.

**Trajectory angle for the brownian case for the *linear transitions dichotomous* (LTD) potential**

In the main text we gave the analytical expression for the trajectory angle in the deterministic limit for the LTD potential. Here we give the expression for the general case, including the effect of Brownian motion. The LTD potential can be written as (see inset in Fig. 2 in the article):

$$\tilde{\mathcal{A}}(\tilde{x}) = \begin{cases} 0 & 0 \leq \tilde{x} \leq \epsilon_1 \\ \tilde{\mathcal{F}}_{max}(\tilde{x} - \epsilon_1) & \epsilon_1 \leq \tilde{x} \leq \epsilon_1 + \delta \\ 1 & \epsilon_1 + \delta \leq \tilde{x} \leq 1 - \delta \\ -\tilde{\mathcal{F}}_{max}(\tilde{x} - 1) & 1 - \delta \leq \tilde{x} \leq 1 \end{cases},$$

where $\tilde{\mathcal{F}}_{max} = 1/\delta$ is the dimensionless maximum force. We note that the width of the regions of constant potential are related by $\epsilon_2 = 1 - \epsilon_1 - 2\delta$. Substituting the above form of the potential into Eq. (5) in the main text,

$$\tan\theta = \tan\theta_F \left[ \frac{\mathrm{Pe}}{1 - e^{-\mathrm{Pe}}} \int_0^1 d\tilde{x}\, e^{-\beta\mathcal{A}'(\tilde{x})} \int_{\tilde{x}}^{\tilde{x}+1} d\xi\, e^{\beta\mathcal{A}'(\xi)} \right],$$

where $\beta\mathcal{A}'(\tilde{x}) = \log\mathcal{K}\,\tilde{\mathcal{A}}(\tilde{x}) - \mathrm{Pe}\,\tilde{x}$, we obtain the analytical expression for the trajectory angle in the general case:

$$\tan\theta = \tan\theta_F \frac{S}{\mathrm{Pe}\,(1 - e^{-\mathrm{Pe}})},$$

where

$$S = \left(1 - e^{-\mathrm{Pe}}\right) \sum_{i=1}^{4} J_i + \sum_{i=1}^{4} \sum_{j=i}^{4} I_{p_i} I_{m_j} + \sum_{i=1}^{3} I_i.$$

The terms in the summations above come from integrals in Eq. (5) that have been combined and rearranged in order to be able to express them in a form that can be readily evaluated for the cases in which $f \neq 1$ and $f = 1$. The definition of $J_i$, $I_i$, $I_{p_i}$, and $I_{m_i}$ are given below for both $f \neq 1$ and $f = 1$.

**$f \neq 1$ case:**

$$J_1 = \mathrm{Pe}\,\epsilon_1 - \left(1 - e^{-\mathrm{Pe}\,\epsilon_1}\right)$$

$$J_2 = \frac{f}{f-1} \left[ \mathrm{Pe}\,\delta - \frac{f}{f-1} \left(1 - \mathcal{K} e^{-\mathrm{Pe}\,\delta}\right) \right]$$

$$J_3 = \mathrm{Pe}\,\epsilon_2 - \left[1 - e^{-\mathrm{Pe}\,\epsilon_2}\right]$$

$$J_4 = \frac{f}{f+1} \left[ \mathrm{Pe}\,\delta - \frac{f}{f+1} \left(1 - \frac{1}{\mathcal{K}} e^{-\mathrm{Pe}\,\delta}\right) \right]$$

$$I_{m_1} = e^{-\mathrm{Pe}\,(1-\epsilon_1)}\left(1 - e^{-\mathrm{Pe}\,\epsilon_1}\right)$$

$$I_{m_2} = \frac{f}{f-1} e^{-\mathrm{Pe}\,(\epsilon_2+\delta)}\left(\frac{1}{\mathcal{K}} - e^{-\mathrm{Pe}\,\delta}\right)$$

$$I_{m_3} = \frac{1}{\mathcal{K}} e^{-\mathrm{Pe}\,\delta}\left(1 - e^{-\mathrm{Pe}\,\epsilon_2}\right)$$

$$I_{m_4} = \frac{f}{f+1}\left(1 - \frac{1}{\mathcal{K}} e^{-\mathrm{Pe}\,\delta}\right)$$

$$I_{p_1} = 1 - e^{-\mathrm{Pe}\,\epsilon_1}$$

$$I_{p_2} = \frac{f}{f-1} e^{-\mathrm{Pe}\,\epsilon_1}\left(1 - \mathcal{K} e^{-\mathrm{Pe}\,\delta}\right)$$

$$I_{p_3} = \mathcal{K} e^{-\mathrm{Pe}\,(\epsilon_1+\delta)}\left(1 - e^{-\mathrm{Pe}\,\epsilon_2}\right)$$

$$I_{p_4} = \frac{f}{f+1} e^{-\mathrm{Pe}\,(1-\delta)}\left(\mathcal{K} - e^{-\mathrm{Pe}\,\delta}\right)$$

$$I_1 = \frac{f}{f-1}\left(1 - \mathcal{K} e^{-\mathrm{Pe}\,\delta}\right)\left(1 - e^{-\mathrm{Pe}\,\epsilon_1}\right)$$

$$I_2 = \mathcal{K}\frac{f}{f-1}\left(1 - e^{-\mathrm{Pe}\,\epsilon_2}\right)\left[\frac{1}{\mathcal{K}} - e^{-\mathrm{Pe}\,(\epsilon_1+\delta)} - e^{-\mathrm{Pe}\,\delta}\left(1 - e^{-\mathrm{Pe}\,\epsilon_1}\right)\frac{1}{f}\right]$$

$$I_3 = \frac{f}{f+1}\left(\mathcal{K} - e^{-\mathrm{Pe}\,\delta}\right)\left[e^{-\mathrm{Pe}\,(\epsilon_2+\delta)}\left(1 - e^{-\mathrm{Pe}\,\epsilon_1}\right) + \frac{f}{f-1} e^{-\mathrm{Pe}\,\epsilon_2}\left(\frac{1}{\mathcal{K}} - e^{-\mathrm{Pe}\,\delta}\right) + \frac{1}{\mathcal{K}}\left(1 - e^{-\mathrm{Pe}\,\epsilon_2}\right)\right]$$

$f = 1$ **case:**

$$J_1 = \mathrm{Pe}\,\epsilon_1 - \left(1 - e^{-\mathrm{Pe}\,\epsilon_1}\right)$$

$$J_2 = \frac{1}{2}\left(\mathrm{Pe}\,\delta\right)^2$$

$$J_3 = \mathrm{Pe}\,\epsilon_2 - \left(1 - e^{-\mathrm{Pe}\,\epsilon_2}\right)$$

$$J_4 = \frac{1}{4}\left(-1 + 2\mathrm{Pe}\,\delta + e^{-2\mathrm{Pe}\,\delta}\right)$$

$$I_{m_1} = e^{-\mathrm{Pe}\,(1-\epsilon_1)}\left(1 - e^{-\mathrm{Pe}\,\epsilon_1}\right)$$

$$I_{m_2} = \mathrm{Pe}\,\delta e^{-\mathrm{Pe}\,(1-\epsilon_1)}$$

$$I_{m_3} = e^{-2\mathrm{Pe}\,\delta}\left(1 - e^{-\mathrm{Pe}\,\epsilon_2}\right)$$

$$I_{m_4} = \frac{1}{2}\left(1 - e^{-2\mathrm{Pe}\,\delta}\right)$$

$$I_{p_1} = 1 - e^{-\mathrm{Pe}\,\epsilon_1}$$

$$I_{p_2} = \mathrm{Pe}\,\delta e^{-\mathrm{Pe}\,\epsilon_1}$$

$$I_{p_3} = e^{-\mathrm{Pe}\,\epsilon_1}\left(1 - e^{-\mathrm{Pe}\,\epsilon_2}\right)$$

$$I_{p_4} = \frac{1}{2}e^{-\mathrm{Pe}\,(1-2\delta)}\left(1 - e^{-2\mathrm{Pe}\,\delta}\right)$$

$$I_1 = \mathrm{Pe}\,\delta\left(1 - e^{-\mathrm{Pe}\,\epsilon_1}\right)$$

$$I_2 = \left(1 - e^{-\mathrm{Pe}\,\epsilon_2}\right)\left(1 + \mathrm{Pe}\,\delta - e^{-\mathrm{Pe}\,\epsilon_1}\right)$$

$$I_3 = \frac{1}{2}\left(1 - e^{-2\mathrm{Pe}\,\delta}\right)\left[1 + e^{-\mathrm{Pe}\,\epsilon_2}\left(\mathrm{Pe}\,\delta - e^{-\mathrm{Pe}\,\epsilon_1}\right)\right]$$

# References


[1] Salman S Rogers, Thomas A Waigh, Xiubo Zhao, and Jian R Lu. Precise particle tracking against a complicated background: polynomial fitting with gaussian weight. *Physical Biology*, 4:220–227, October 2007.

[2] Natalia Kozlova and Maria M. Santore. Manipulation of Micrometer-Scale adhesion by tuning Nanometer-Scale surface features. *Langmuir*, 22(3):1135–1142, October 2006.

[3] Hung-Jen Wu, W. Neil Everett, Samartha G. Anekal, and Michael A. Bevan. Mapping patterned potential energy landscapes with diffusing colloidal probes. *Langmuir*, 22(16):6826–6836, September 2011.
